# Supplementary material for: FRIEDA: Benchmarking Multi-Step Cartographic Reasoning in Vision-Language Models
Source: arXiv:2512.08016 source file (2026-02-27)
Supplement: Supplementary file 1 [file data-sheet.tex]

\section{Data Sheet}
We follow the documentation framework provided by \cite{c:gebru2021datasheet}.

% https://github.com/TristaCao/into_inclusivecoref/blob/master/GICoref/datasheet-gicoref.md

\subsection{Motivation}

\paragraph{For what purpose was the dataset created?}

\subsection{Composition}

\subsection{Collection Process}

\subsection{Preprocessing/cleaning/labeling}

\subsection{Uses}

\subsection{Distribution}

\subsection{Maintenance}
